# Supplementary material for: A Large-Scale Empirical Comparison of Static and Dynamic Test Case Prioritization Techniques
Source: arXiv:1801.05917 source file (2018-01-18)
Supplement: Supplementary file 1 [file appendix.tex]

% !TEX root = main.tex
\appendix
Table~\ref{tab:comparison} shows the comparison between different test prioritization papers.
\begin{table*}
\center\caption{\label{tab:comparison}The comparison between different test prioritization papers. The first section shows the papers for static techniques, the second section shows the papers for dynamic techniques, and the third section shows the empirical studies for test prioritization techniques.}
\vspace{-0.3cm}
\begin{tabular}{|l||c|c|c|c|c|}
\hline
Papers&Brief Description&Inputs&Compared Techniques&Metrics&Subject projects\\\hline\hline
\multirow{2}{*}
{Zhang \emph{et. al}~\cite{Zhang:ICSM09}}&Call-graph&test code,&Random, untreated, &APFD&Ant\\
&based&source code&method-add/total&&JTopas\\
\hline
\multirow{2}{*}
{Ledru \emph{et. al}~\cite{Ledru:ASE12}}&String-&test&Random,&APFD&Seven\\
&based&code&different string distances&&C programs\\
\hline
\multirow{2}{*}
{Thomas \emph{et. al}~\cite{Thomas:EMSE14}}&Topic-&test&Random, String/call-&APFD&Ant\\
&based&code&graph-based&&Derby\\
\hline
\multirow{2}{*}
{Jiang \emph{et. al}~\cite{Jiang:compsac13}}&Input-&test code, source&Random, statement/brach&APFD,&Four Unix\\
&based&code,inputs&/method-add/total&ANOVA&programs\\
\hline
\multirow{2}{*}
{Saha \emph{et. al}~\cite{Saha:ICSE15}}&Change-based,&test code, source&Random, call-graph, me-&APFD&Versions of eight\\
&VSM&code, changes&thod/statement-add/total&&Java programs\\
\hline
\hline
\hline
\multirow{2}{*}
{Walcott \emph{et. al}~\cite{Walcott:06}}&Genetic algorithm,&Coverage,&Coverage&APFD&Gradebook,\\
&time constraints&execution time&-total&&JDepend\\
\hline
\multirow{2}{*}
{Li \emph{et. al}~\cite{Li:07}}&Coverage-based,&Coverage&Block/statement&APFD,&Six\\
&GA&&-addi/total&average coverage&C programs\\
\hline
\multirow{2}{*}
{Islam \emph{et. al}~\cite{Islam:CSMR12}}&Coverage, LSI,&Coverage, require-&Random, statement&APFD&AveCalc,\\
&requirement, GA&ments, source code&-addi/total&&LaTazza\\
\hline
\multirow{2}{*}
{Zhang \emph{et. al}~\cite{zhang2013bridging}}&Bridge gap between&Coverage&Method/statement&APFD&Versions of four\\
&total and additional&&-addi/total&&Java programs\\
\hline
\hline
\hline
\multirow{2}{*}
{Rothermel \emph{et. al}~\cite{Rothermel:99}}&Study (the effectiveness for &Coverage, probabilities of&Random, optimal, different&APFD&Seven\\
&improving fault detection)&fault existence/exposure&inputs*different granularity&&C programs\\
\hline
\multirow{2}{*}
{Elbaum \emph{et. al}~\cite{Elbaum:TSE02}}&Study (Versions, types of&Coverage, probabilities of&Random, optimal, different&APFD&Eight\\
&programs, granularity, etc.)&fault existence/exposure&inputs*different granularity&&C programs\\
\hline
\multirow{2}{*}
{Do \emph{et. al}~\cite{Do:04}}&Study (whether TP techniques&Coverage with diff&Random, optimal, different&APFD&Ant, XML\\
&also work on Java programs)&-erent granularity&inputs*different granularity&&JMeter, JTopas\\
\hline
\multirow{2}{*}
{Elbaum \emph{et. al}~\cite{Elbaum:SQI04}}&Study (various attributes of&Coverage&Random, optimal,&APFD,&Eight\\
&programs, modifications)&&coverage-total/additional&diff in APFD&C programs\\
\hline
\multirow{2}{*}
{Qu \emph{et. al}~\cite{Qu:ISSTA08}}&Study (the configurations,&Coverage, fault detection&Different inputs&NAPFD&Different ver-\\
&of a software system)&change across faults&*different granularity&&sions of vim\\
\hline
\multirow{2}{*}
{Smith \emph{et. al}~\cite{Smith:SAC09}}&Study (test cost, &Coverage, test&Different greedy TP&Coverage&Eight Java\\
&test effectiveness)&execution time&and RTM techniques&Effectiveness&programs\\
\hline
\end{tabular}
\end{table*}
